# Supplementary material for: Automatic Digitization and Orientation of Scanned Mesh Data for Floor Plan and 3D Model Generation
Source: arXiv:2311.11927 source file (2023-11-15)
Supplement: Supplementary file 1 [file 6-supplementarymaterial.tex]

\newpage
\clearpage
\section*{Supplemental Materials}
Due to the space limitation in the manuscript, we include additional algorithms and figures in this supplemental section.

\subsection*{Orienting the floor using a bounding box}
It is often the case that one story of a building will be larger horizontally than vertically, that the ceiling will be at a constant altitude, and that the floor will be at a constant altitude. In this case, a simple bounding box method is enough to orient the mesh $\mathcal{M}$ so that its floor is level (at a constant y value). 

% In this case, we can proceed as follows:

\vspace{-0.3cm}
\begin{algorithm}
\caption{Orienting the floor using the bounding box method}
\begin{algorithmic}[1]
  \State $\mathcal{BB}~\gets$ \textit{ComputeBoundingBox}$(\mathcal{M})$;
  \State $\vec{g_{m}}~\gets$ \textit{ComputeModelGravityFromBox}$(\mathcal{BB})$;
  \State $\vec{g_{t}}~\gets$ -$\vec{y}$;
  \State $\theta~\gets \arccos(\vec{g_{t}}$ . $\vec{g_{m}})$;
  \State $\mathcal{Y}~\gets$ $\vec{g_{t}}$ x $\vec{g_{m}}$;
  \State $\mathcal{M}$~$\gets$ $\textit{rotateMesh}$ $(\theta, \mathcal{Y})$;
\end{algorithmic}
\label{alg:BBMethod}
\end{algorithm}
\vspace{-0.3cm}

To orient the mesh $\mathcal{M}$ based on its bounding box, first, a tightly fitting bounding box $\mathcal{BB}$ is computed. The vertical dimension of the bounding box is assumed to be the minimum dimension. Then, the surface normal of the top face of this bounding box, pointing towards the interior, is calculated to obtain an approximation of the true gravity direction $\vec{g_{m}}$. The angle $\theta$ is computed using the dot product of $\vec{g_{t}}$ and $\vec{g_{m}}$ followed by applying the arccosine function. The axis of rotation $\mathcal{Y}$ is computed by taking the cross product of those vectors. The mesh is then rotated by $\theta$ along the $\mathcal{Y}$ axis, resulting in a horizontal floor. For a more detailed formal description of the bounding box method, please refer to Algorithm~\ref{alg:BBMethod}.

\subsection*{Opacity and Slicing Experiment}
To determine appropriate opacity and slicing, we first varied the opacity across values of 0.1, 0.3, 0.5, 0.7, and 0.9 while keeping the number of slices constant. The results of our opacity test, as shown in Figure~\ref{fig:OpacityTest}, indicate that an opacity of 0.5 yields a satisfactory floor plan. Next, we tested the effect of increasing or decreasing the number of slices used to create a pen-and-ink style floor plan. As we increase the number of slices, more details such as furniture shapes and tabletops become visible. Conversely, reducing the number of slices produces a lighter, less cluttered floor plan. Figure~\ref{fig:slicingTest} illustrates the results of our slicing test. We determined that generating a floor plan with 100 slices balances detail and clutter reduction well, but depending on the use case, other values may be more desirable.

\begin{figure*}[!ht]
  \includegraphics[width=\linewidth]{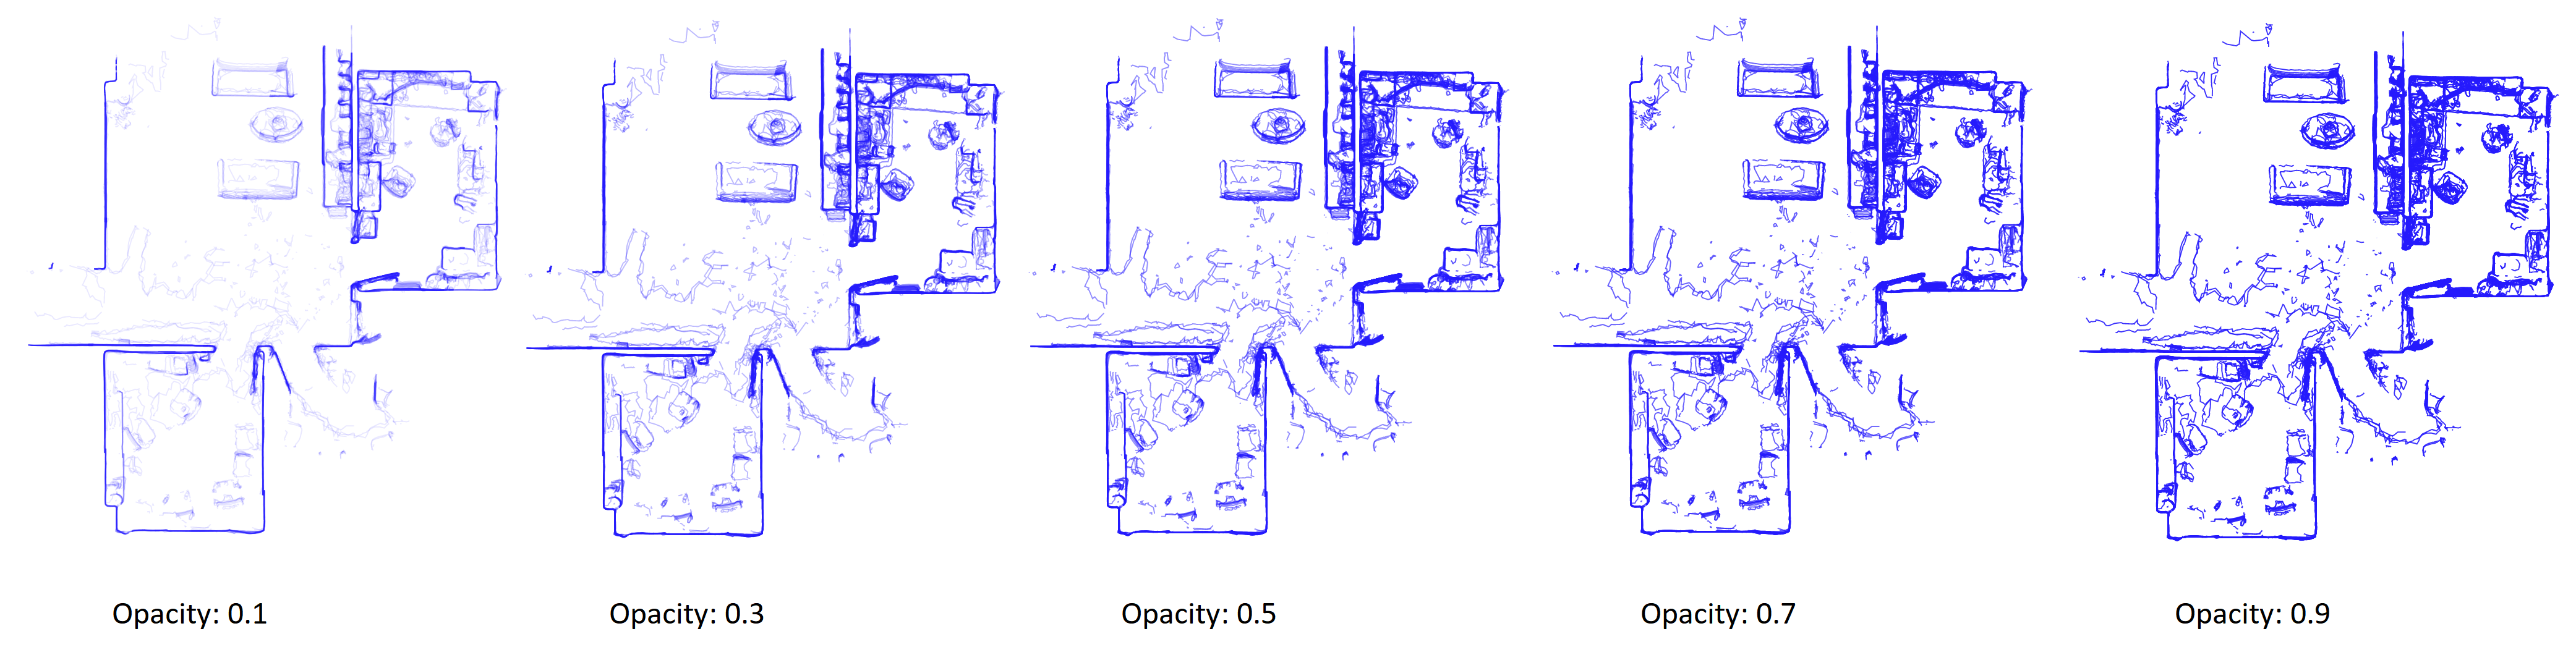}
  \centering
  \caption{Pen-and-ink style floor plans with opacity equal to 0.1, 0.3, 0.5, 0.7 and 0.9 from left to right.}
  \label{fig:OpacityTest}
\end{figure*}
\begin{figure*}[!ht]
  \includegraphics[width=\linewidth]{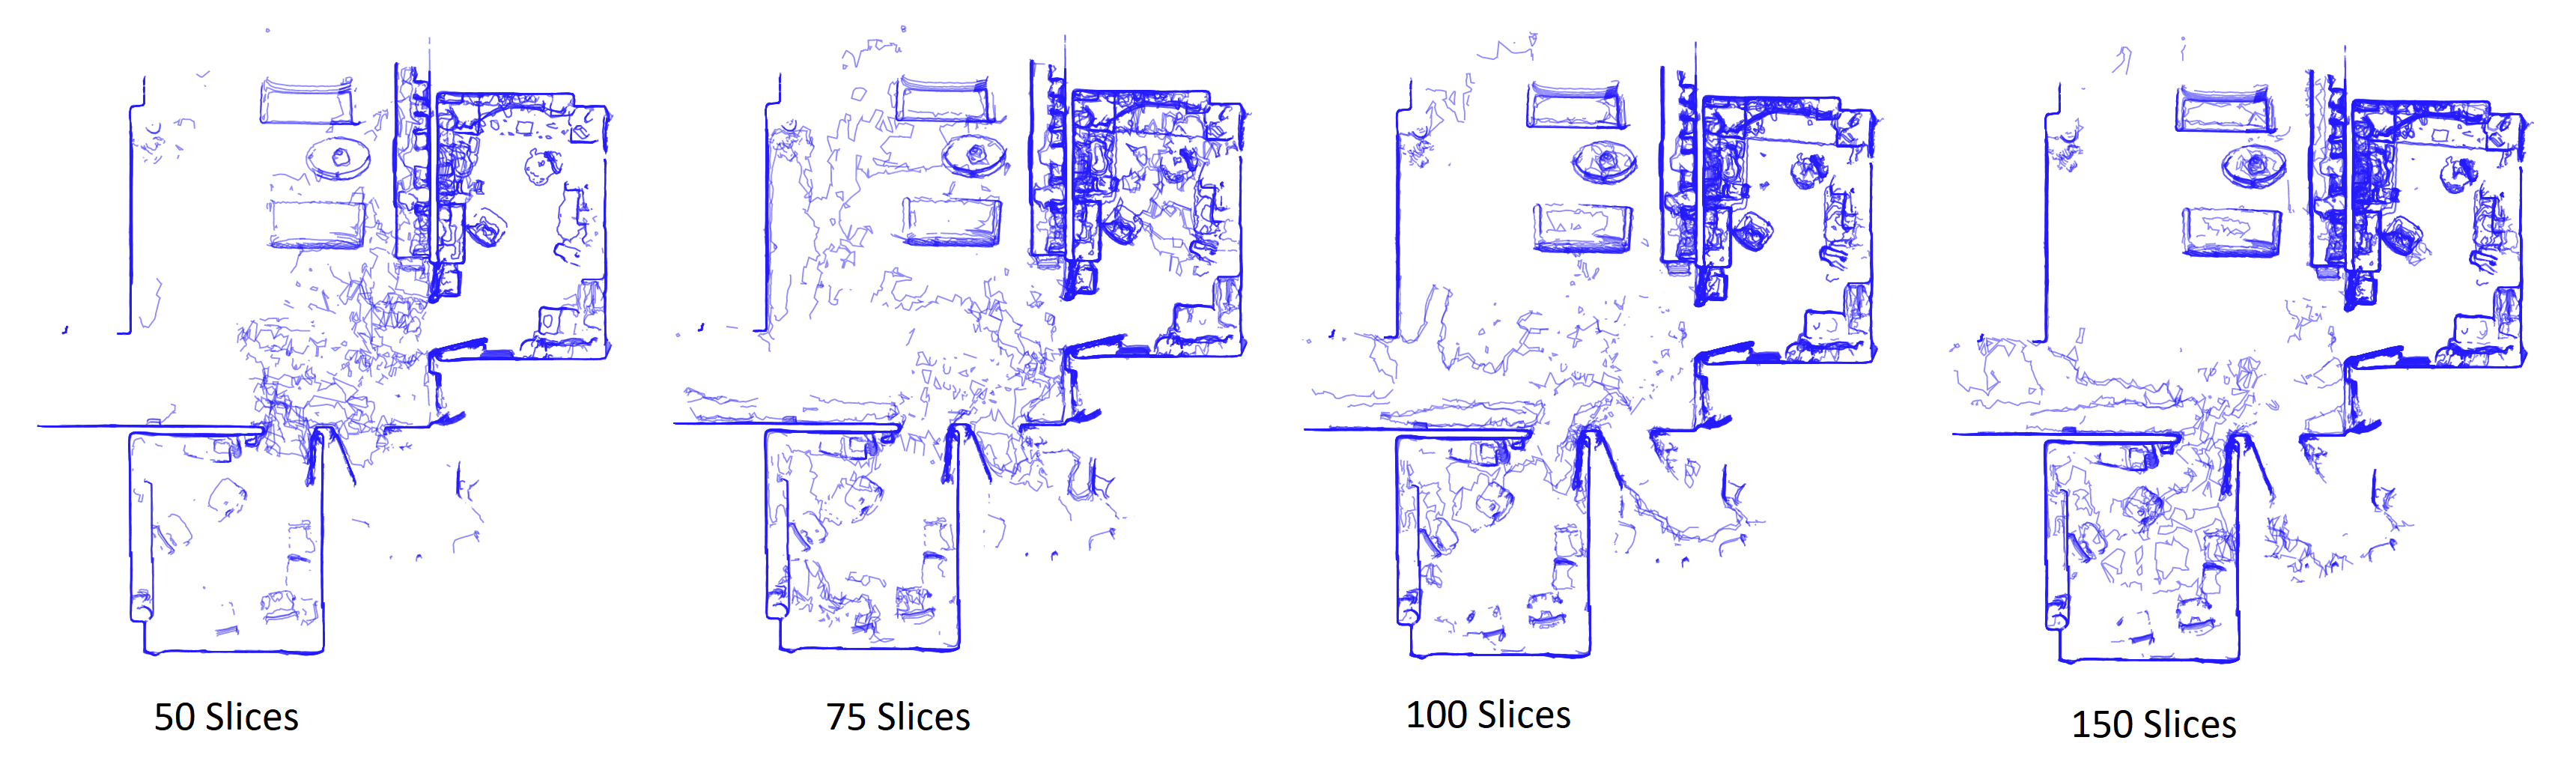}
  \centering
  \caption{Pen-and-ink style floor plans with slice count equal to 50, 75, 100, and, 150 from left to right.}
  \label{fig:slicingTest}
\end{figure*}

\subsection*{Additional results} 
In this section, we present the results obtained from various stages of our approach that led to the computation of floor plans and extraction of flat walls. The computational time for each major step involved in the computation of floor plans and extraction of flat walls is provided in Table~\ref{tab:more_analysis1} and Table~\ref{tab:more_analysis2} for single-story and multi-story buildings, respectively. Models 1, 2, and 3 represent single-story buildings, while models 4 and 5 represent multi-story buildings.

\begin{table}[!ht]
\caption{Computational Times(in Seconds): $T_o$, $T_p$, $T_{D_{fp}}$ are the time for orienting mesh, finding planar walls and, computing drafting style floor plan in seconds for a single story building} %title of the table
\centering % centering table
\begin{tabular}{c | rrr} % creating three columns
\hline\hline %inserting double-line
Model  & $T_o$ & $T_p$ &  $T_{D_{fp}}$\\ \hline
1  & 4.63 & 15.17  &  0.51\\
2  &  1.26 & 10.62 & 0.21  \\ 
3  & 42.77  & 174.19 &  1.14  \\ 
\hline % inserts single-line
\end{tabular}
\label{tab:more_analysis1}
\end{table}

\begin{table}[!ht]
\caption{Computational Times(in Seconds): $T_o$, $T_p$, $T_{pr}$ are the total time for orienting mesh of entire building, finding planar walls, and computing drafting style floor plan in seconds for each level of multistory building} %title of the table
\centering % centering table
\begin{tabular}{c | c | rrr} % creating three columns
\hline\hline %inserting double-line
Model &  level &$T_o$ & $T_p$ &  $T_{D_{fp}}$\\ \hline
4  & 0 & 23.92 & 43.6 &  0.41\\
4  & 1 &   & 39.5  &  0.43\\ \hline
5  & 0 & 41.6 &41.70 & 0.62  \\ 
5  & 1 & & 54.44 & 1.24  \\ 
5  & 2 & & 37.97 & 0.99  \\ 
\hline % inserts single-line
\end{tabular}
\label{tab:more_analysis2}
\end{table}

\begin{figure*}[!ht]
  \includegraphics[width=\linewidth]{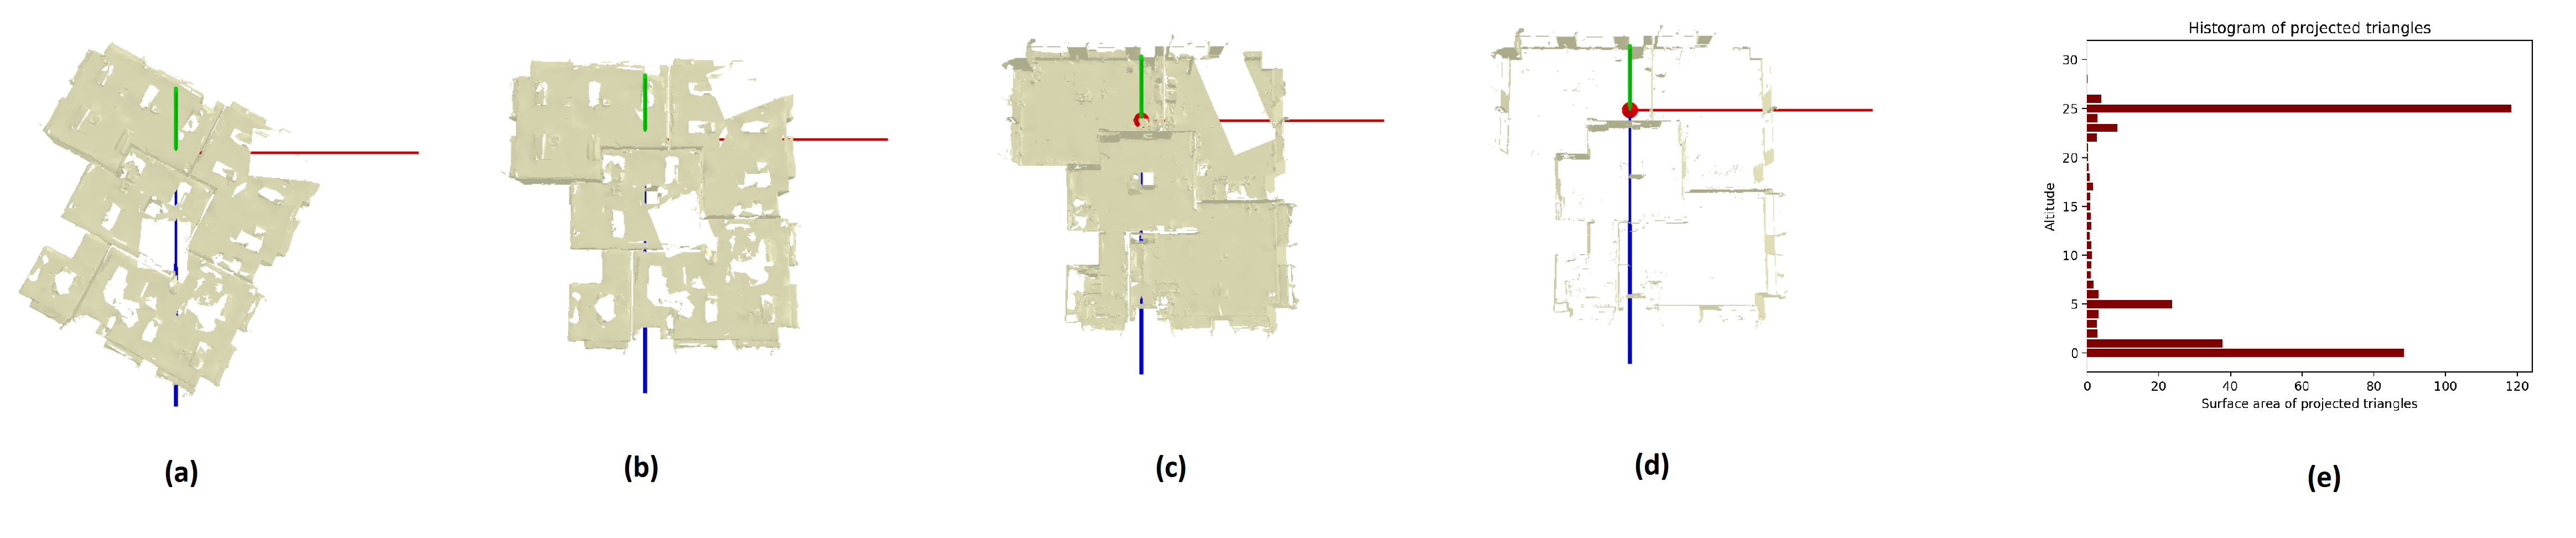}
  \centering
  \caption{ Model 1: (a) Scanned mesh data of a building. (b) Oriented mesh using Spherical K-means. (c,d) Building with ceiling and floor removed respectively. (e) Histogram used for ceiling and floor detection }
  \label{fig:ornl_model1}
\end{figure*}
\begin{figure*}[!ht]
  \includegraphics[width=\linewidth]{cgi2018_latex/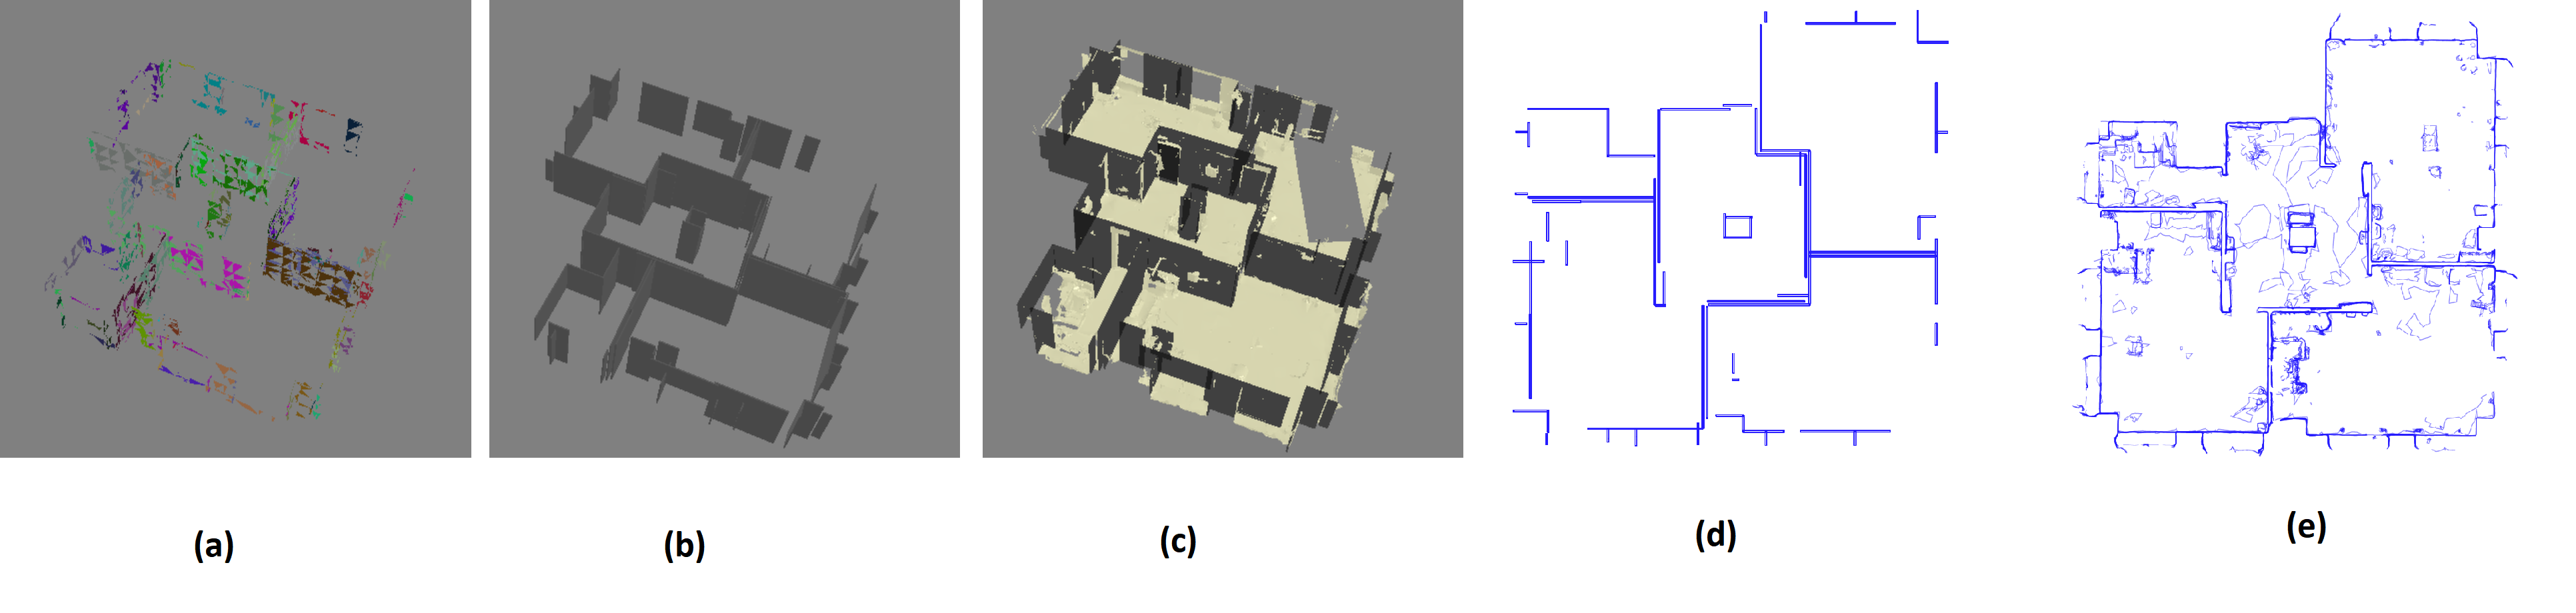}
  \centering
  \caption{Model 1: (a) Cluster obtained using DBSCAN (b) Flat Walls (c) Flat walls with the building model. (d,e) Drafting and Pen-and-Ink style floor plan respectively.}
  \label{fig:ornl_model2}
\end{figure*}

\begin{figure*}[!ht]
  \includegraphics[width=\linewidth]{cgi2018_latex/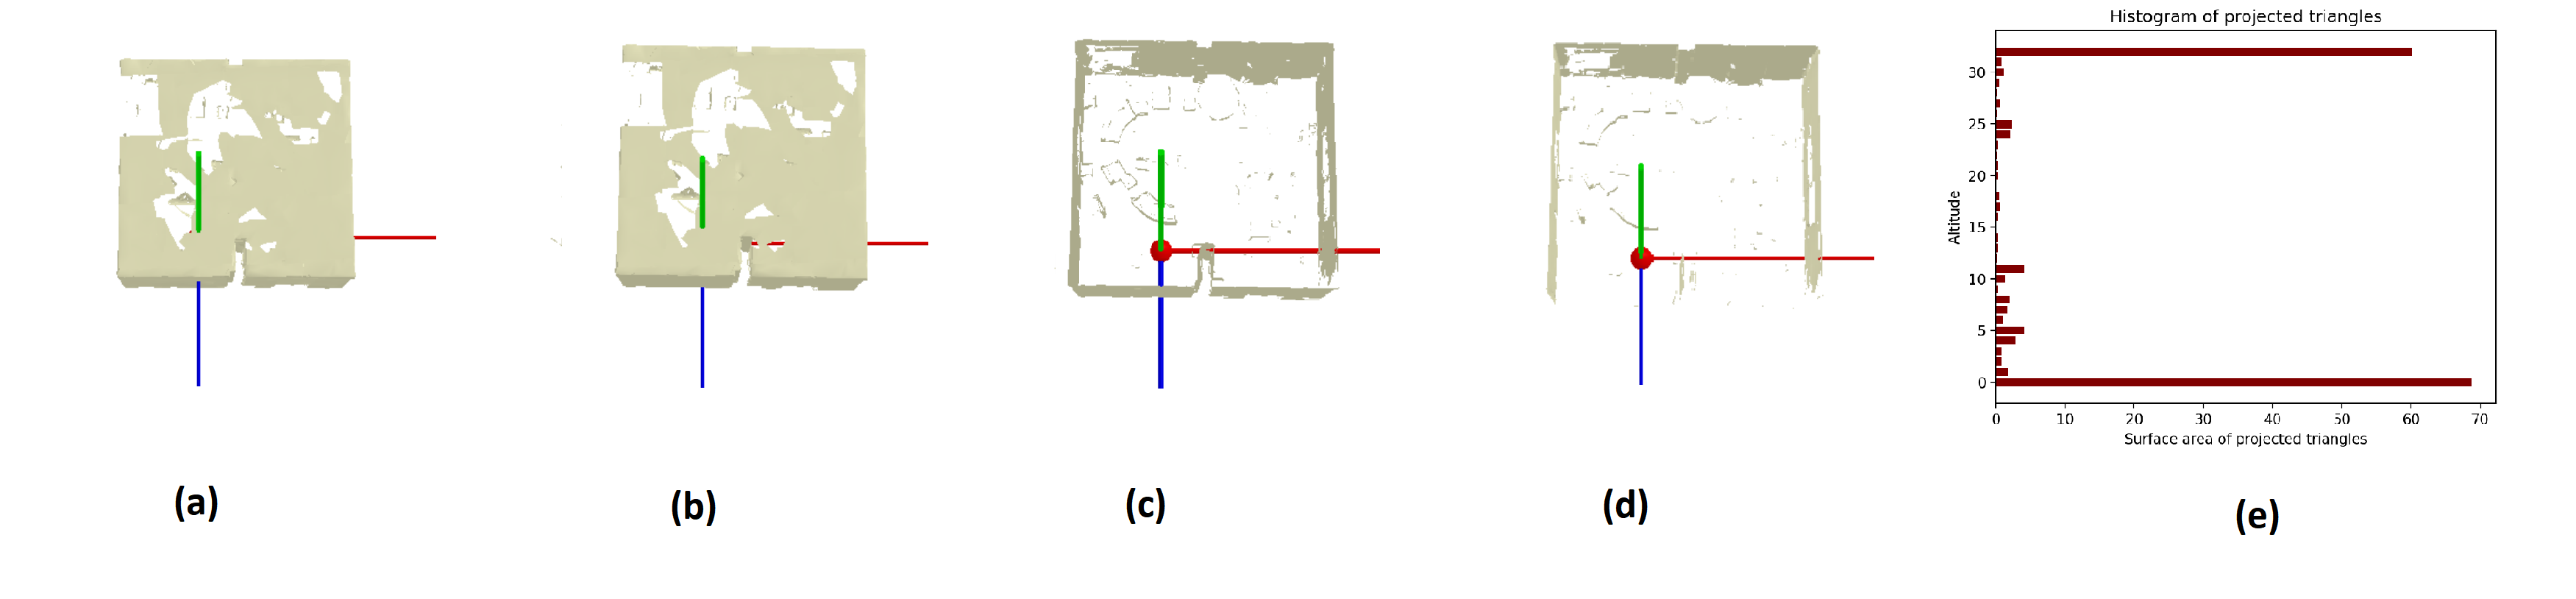}
  \centering
  \caption{Model 2: (a) Scanned mesh data of a building. (b) Oriented mesh using Spherical K-means. (c,d) Building with ceiling and floor removed respectively. (e) Histogram used for ceiling and floor detection }
  \label{fig:model_isg1}
\end{figure*}

\begin{figure*}[!ht]
  \includegraphics[width=\linewidth]{cgi2018_latex/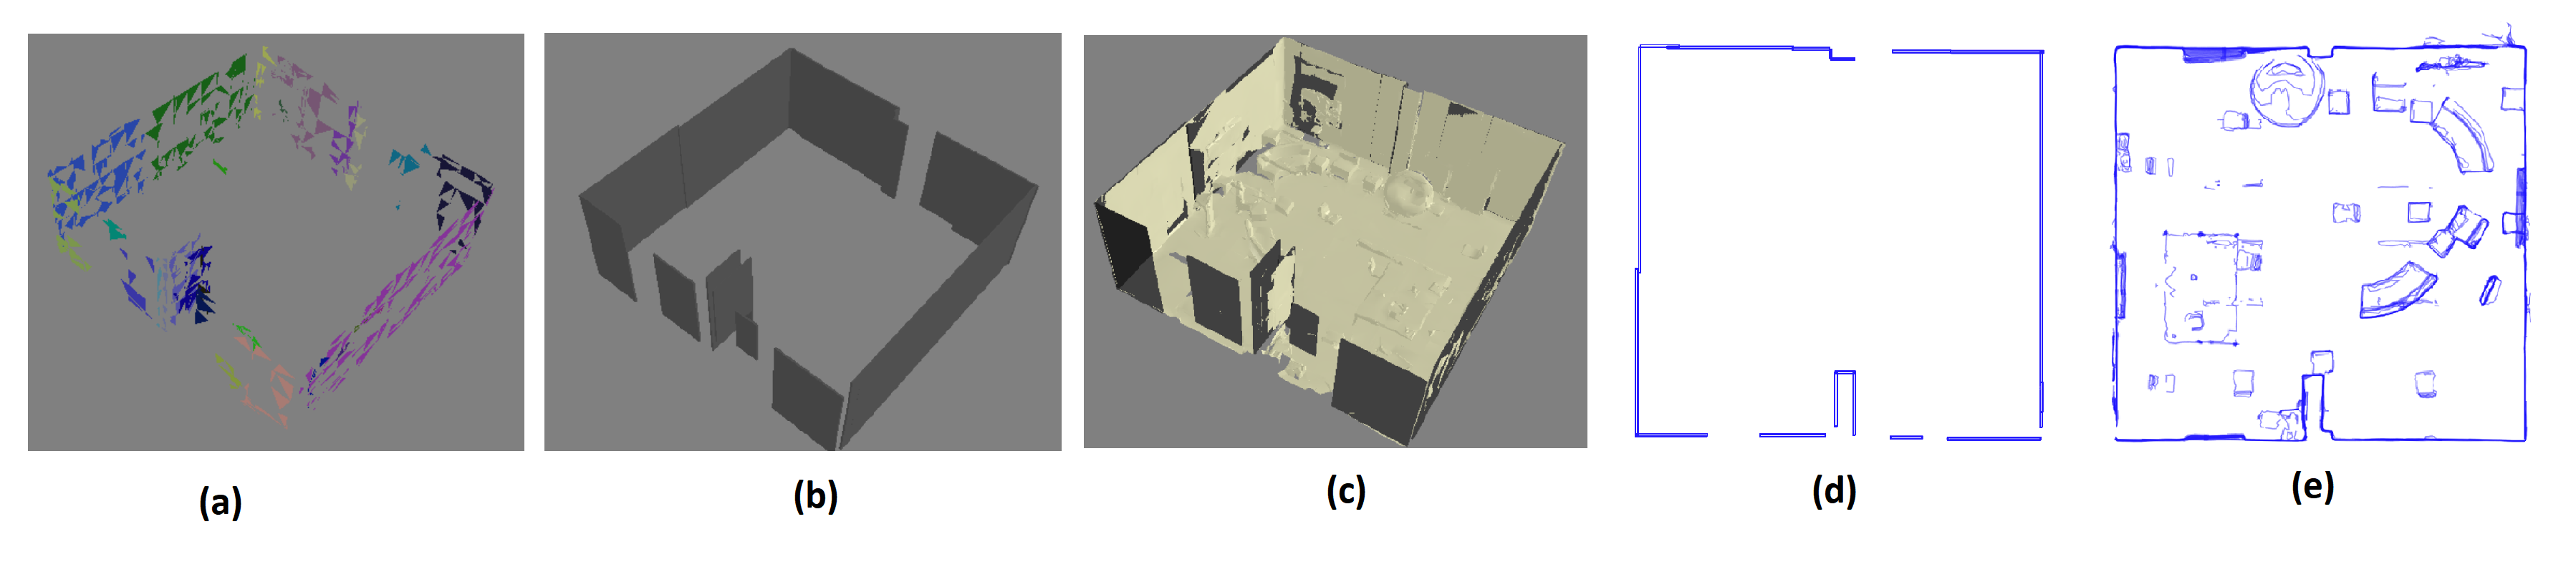}
  \centering
  \caption{Model 2: (a) Cluster obtained using DBSCAN (b) Flat Walls (c) Flat walls with the building model. (d,e) Drafting and Pen-and-Ink style floor plan respectively.}
  \label{fig:model_isg2}
\end{figure*}

\begin{figure*}[!ht]
  \includegraphics[width=\linewidth]{cgi2018_latex/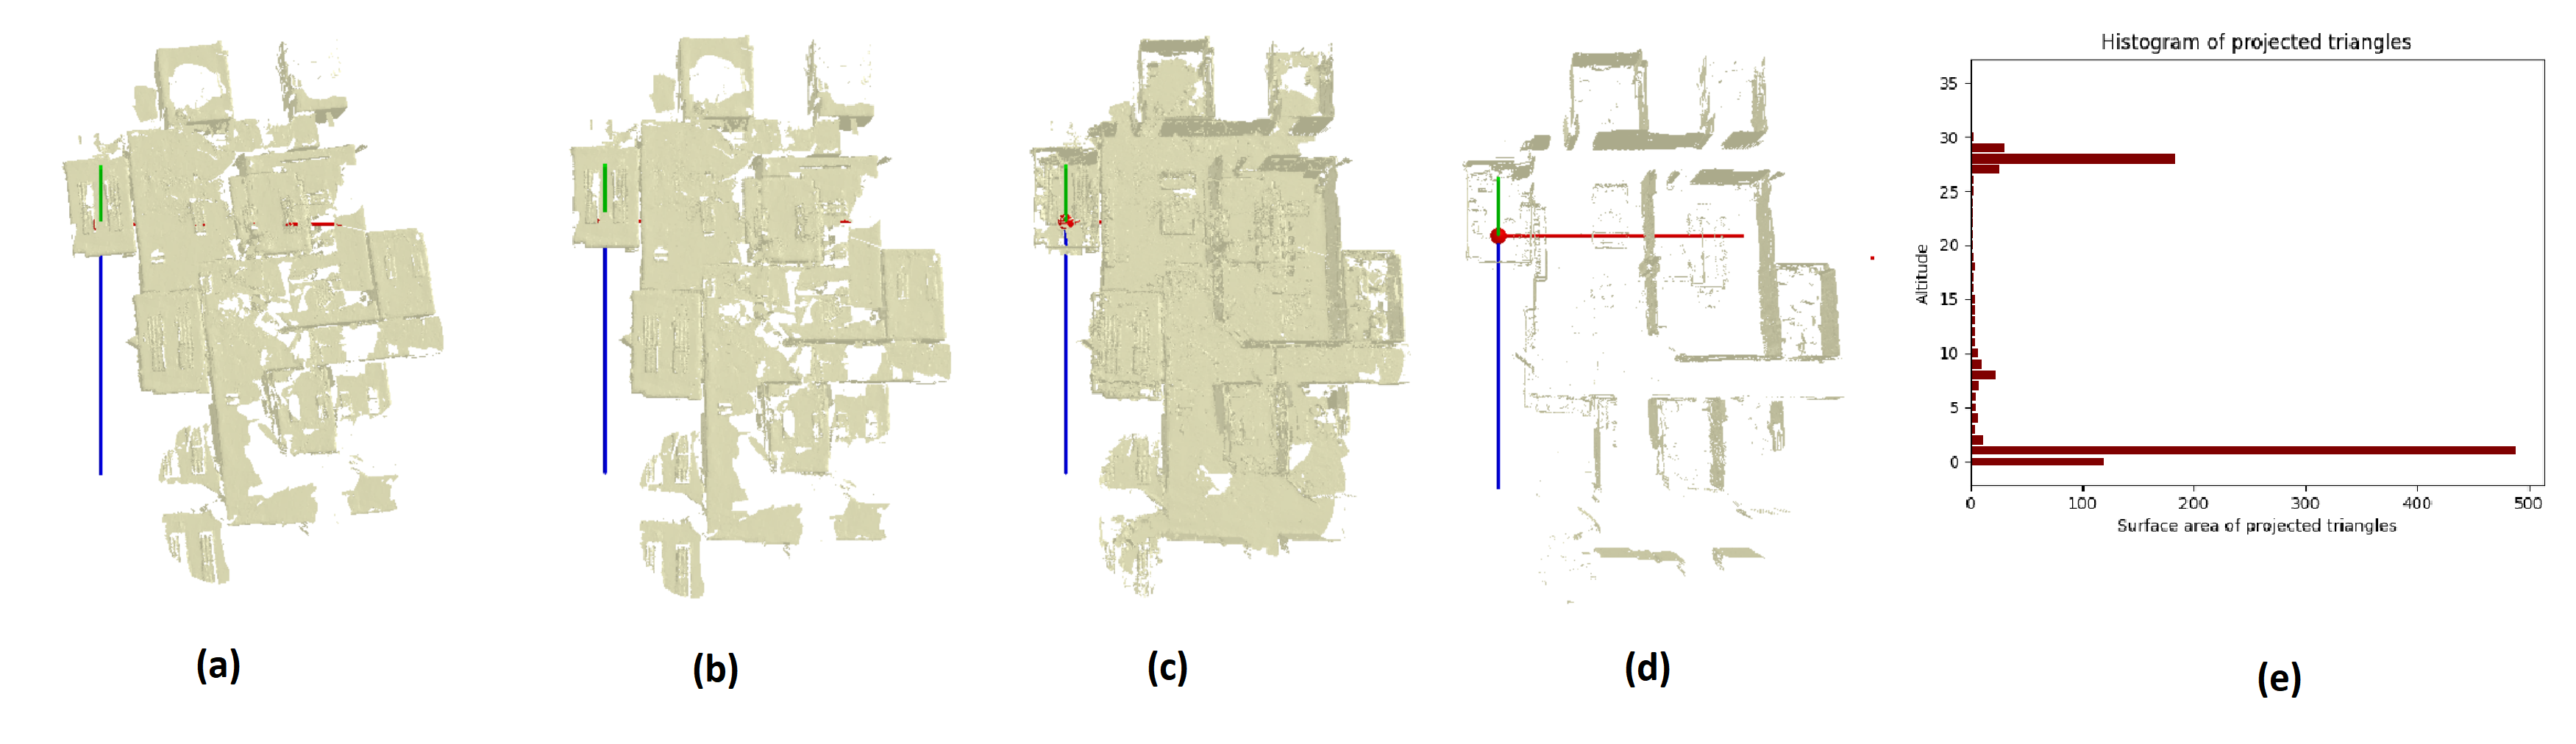}
  \centering
  \caption{Model 3: (a) Scanned mesh data of a building. (b) Oriented mesh using Spherical K-means. (c,d) Building with ceiling and floor removed respectively. (e) Histogram used for ceiling and floor detection }
  \label{fig:Mesh20211021194212_1}
\end{figure*}

\begin{figure*}[!ht]
  \includegraphics[width=\linewidth]{cgi2018_latex/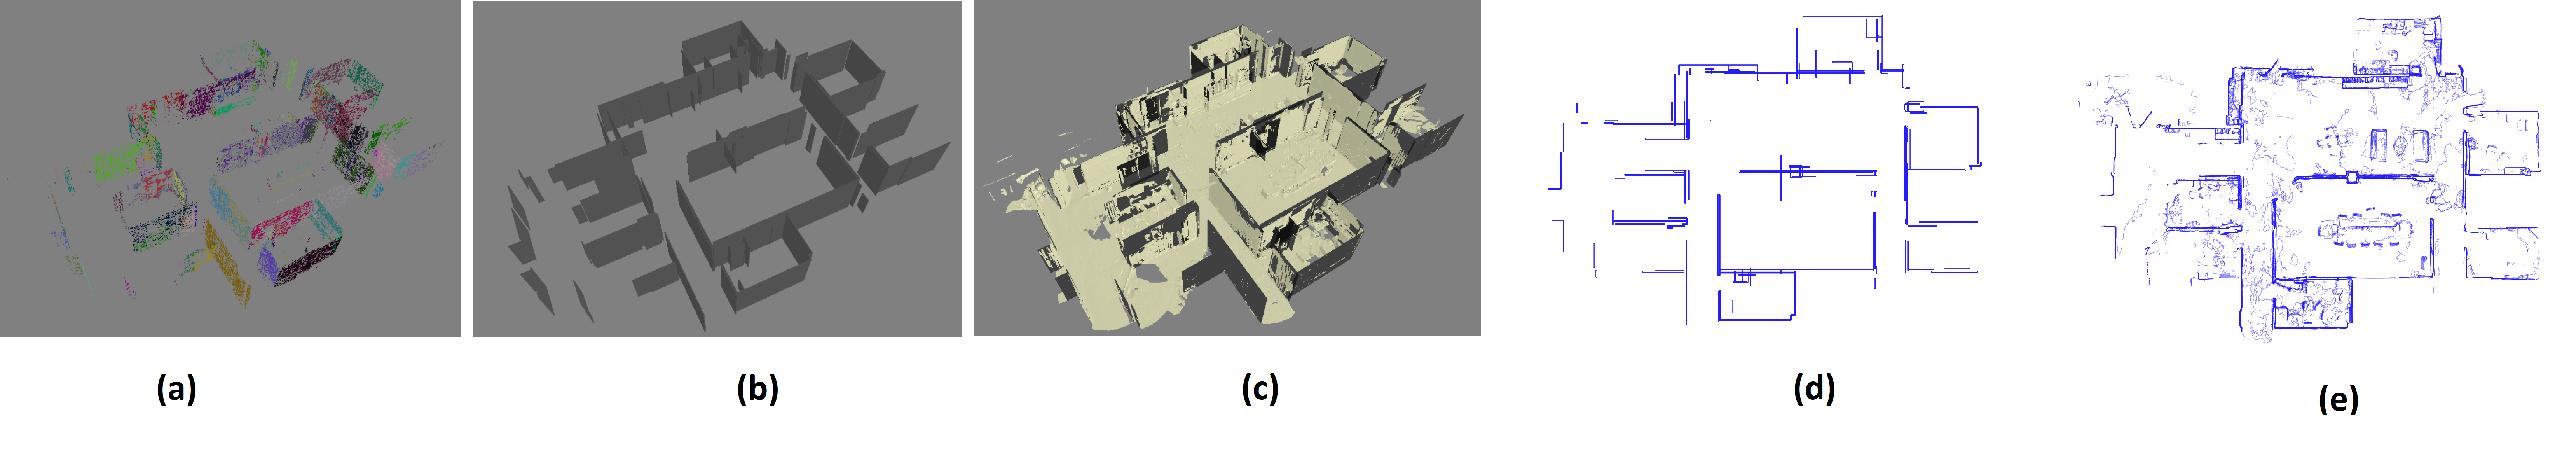}
  \centering
  \caption{Model 3: (a) Cluster obtained using DBSCAN (b) Flat Walls (c) Flat walls with the building model. (d,e) Drafting and Pen-and-Ink style floor plan respectively.}
  \label{fig:Mesh20211021194212_2}
\end{figure*}

\begin{figure*}[!ht]
  \includegraphics[width=\linewidth]{cgi2018_latex/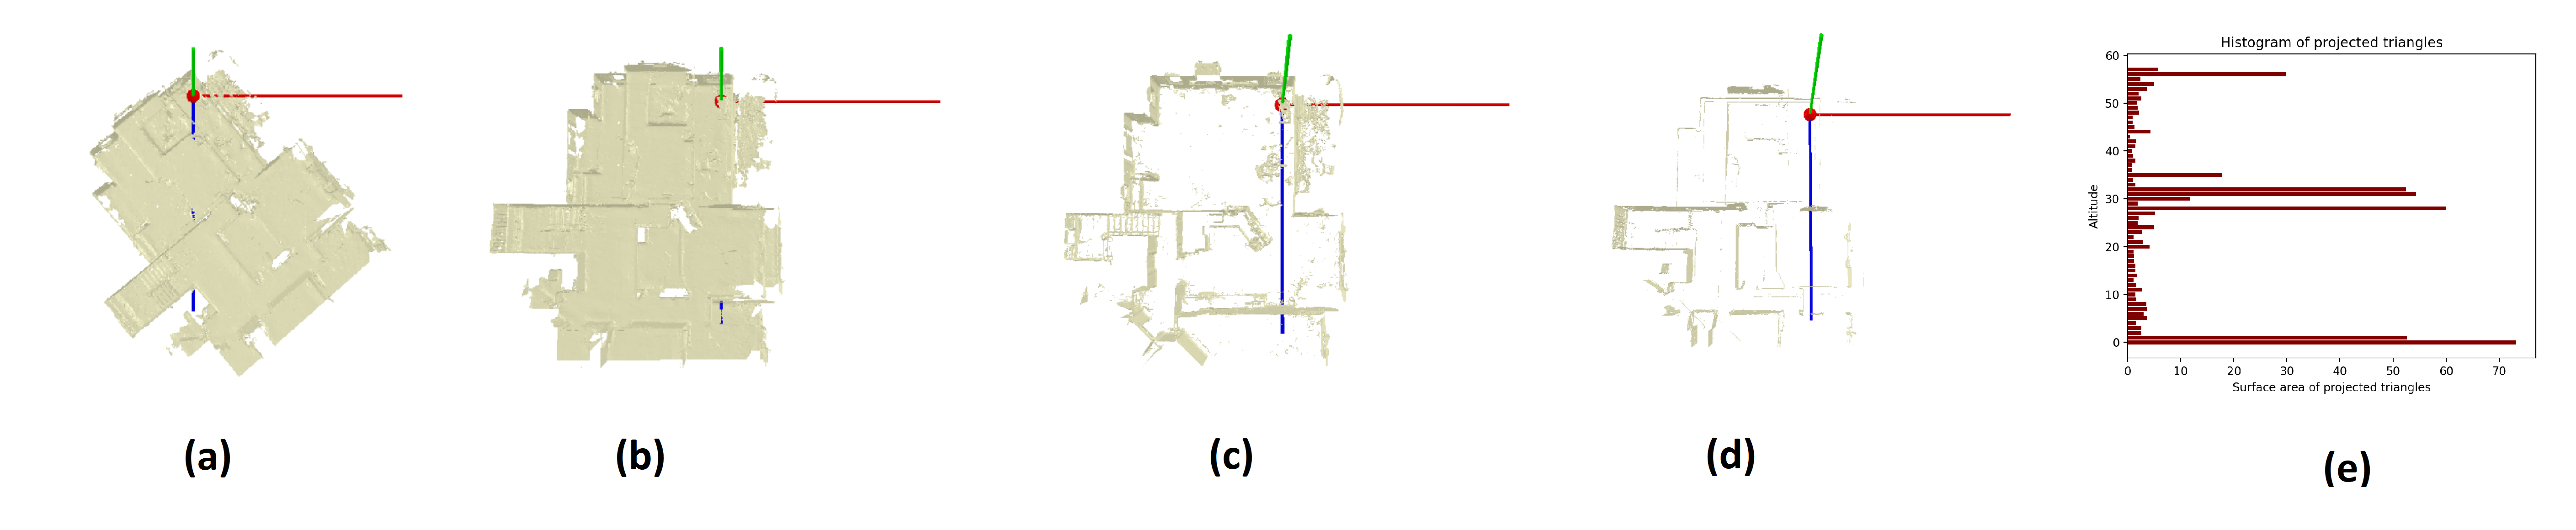}
  \centering
  \caption{Model 4: (a) Scanned mesh data of a two-story building. (b) Oriented mesh using Spherical K-means. (c,d) level 0 and level 1 of the two-story building after partition. (e) Histogram used for partitioning the building }
  \label{fig:LesHouse_level1_level2_1}
\end{figure*}

\begin{figure*}[!ht]
  \includegraphics[width=\linewidth]{cgi2018_latex/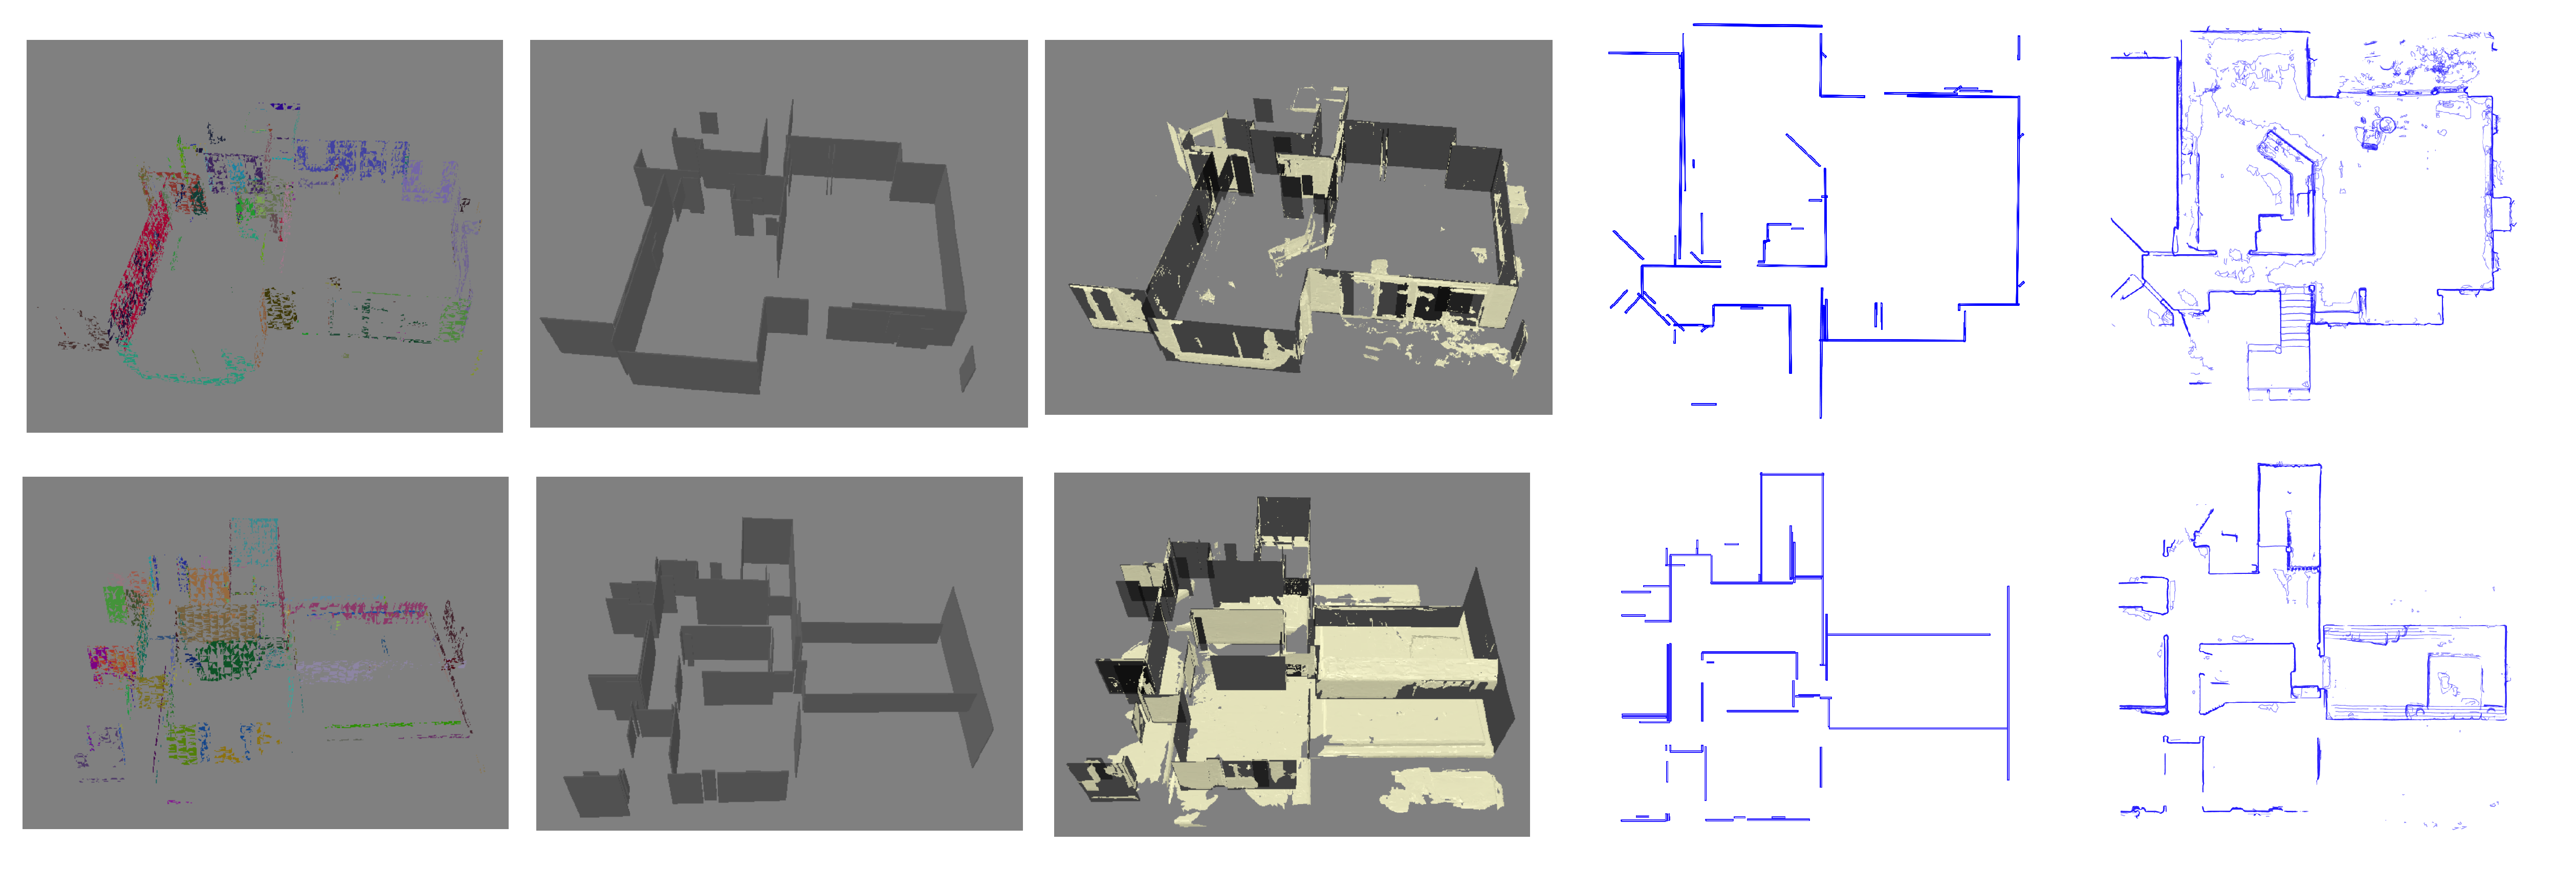}
  \centering
  \caption{Model 4: Left to right: Show clusters, flat walls, flat walls with building, drafting style  and pen-and-ink style floor plan for level 0 (top row) and level 1 (bottom row). }
  \label{fig:LesHouse_level1_level2_2}
\end{figure*}

\begin{figure*}[!ht]
  \includegraphics[width=\linewidth]{cgi2018_latex/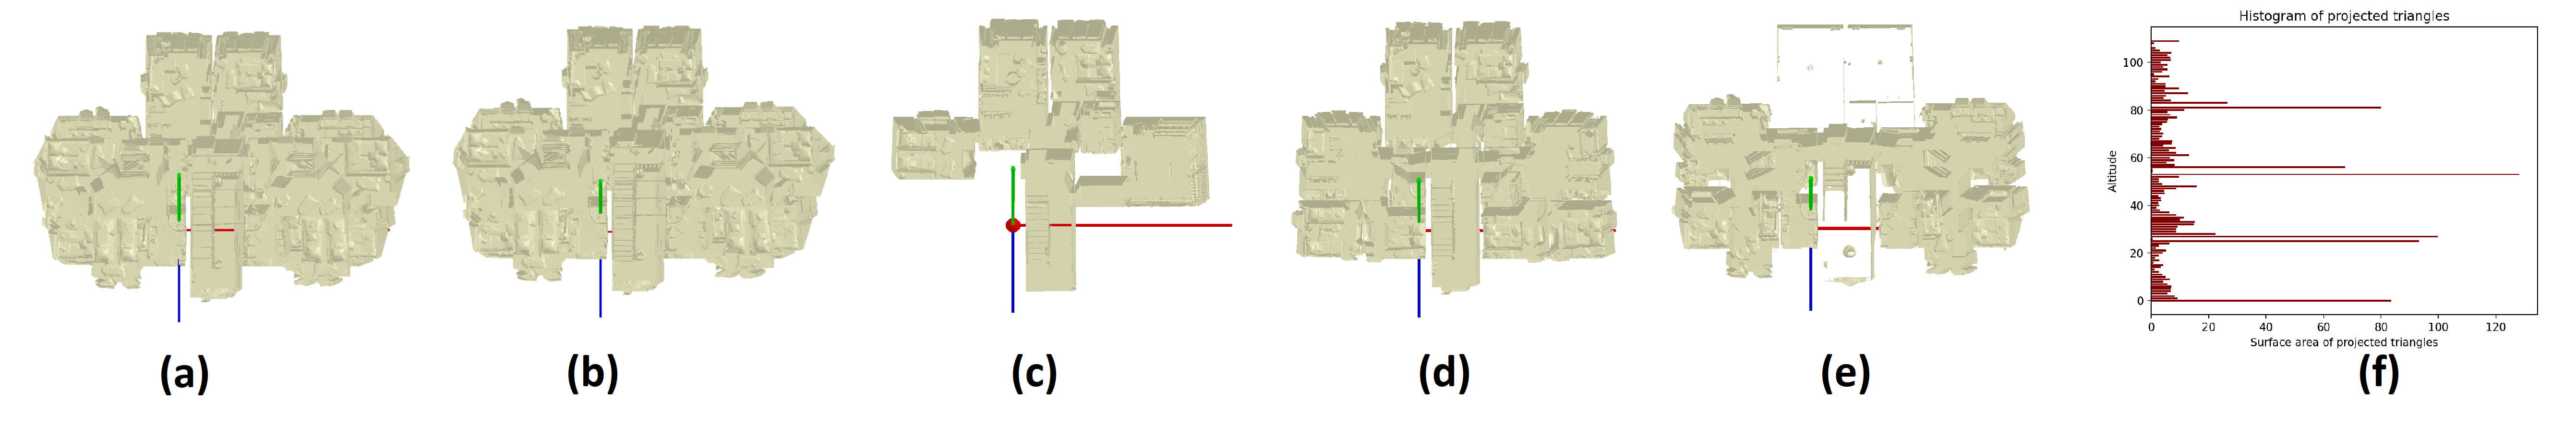}
  \centering
  \caption{Model 5: (a) Scanned mesh data of a three-story building. (b) Oriented mesh using Spherical K-means. (c,d,e) level 0, level 1 and level 2 of the three-story building after partition. (f) Histogram used for partitioning the building }
  \label{fig:matterport_level012_1}
\end{figure*}

\begin{figure*}[!ht]
  \includegraphics[width=\linewidth]{cgi2018_latex/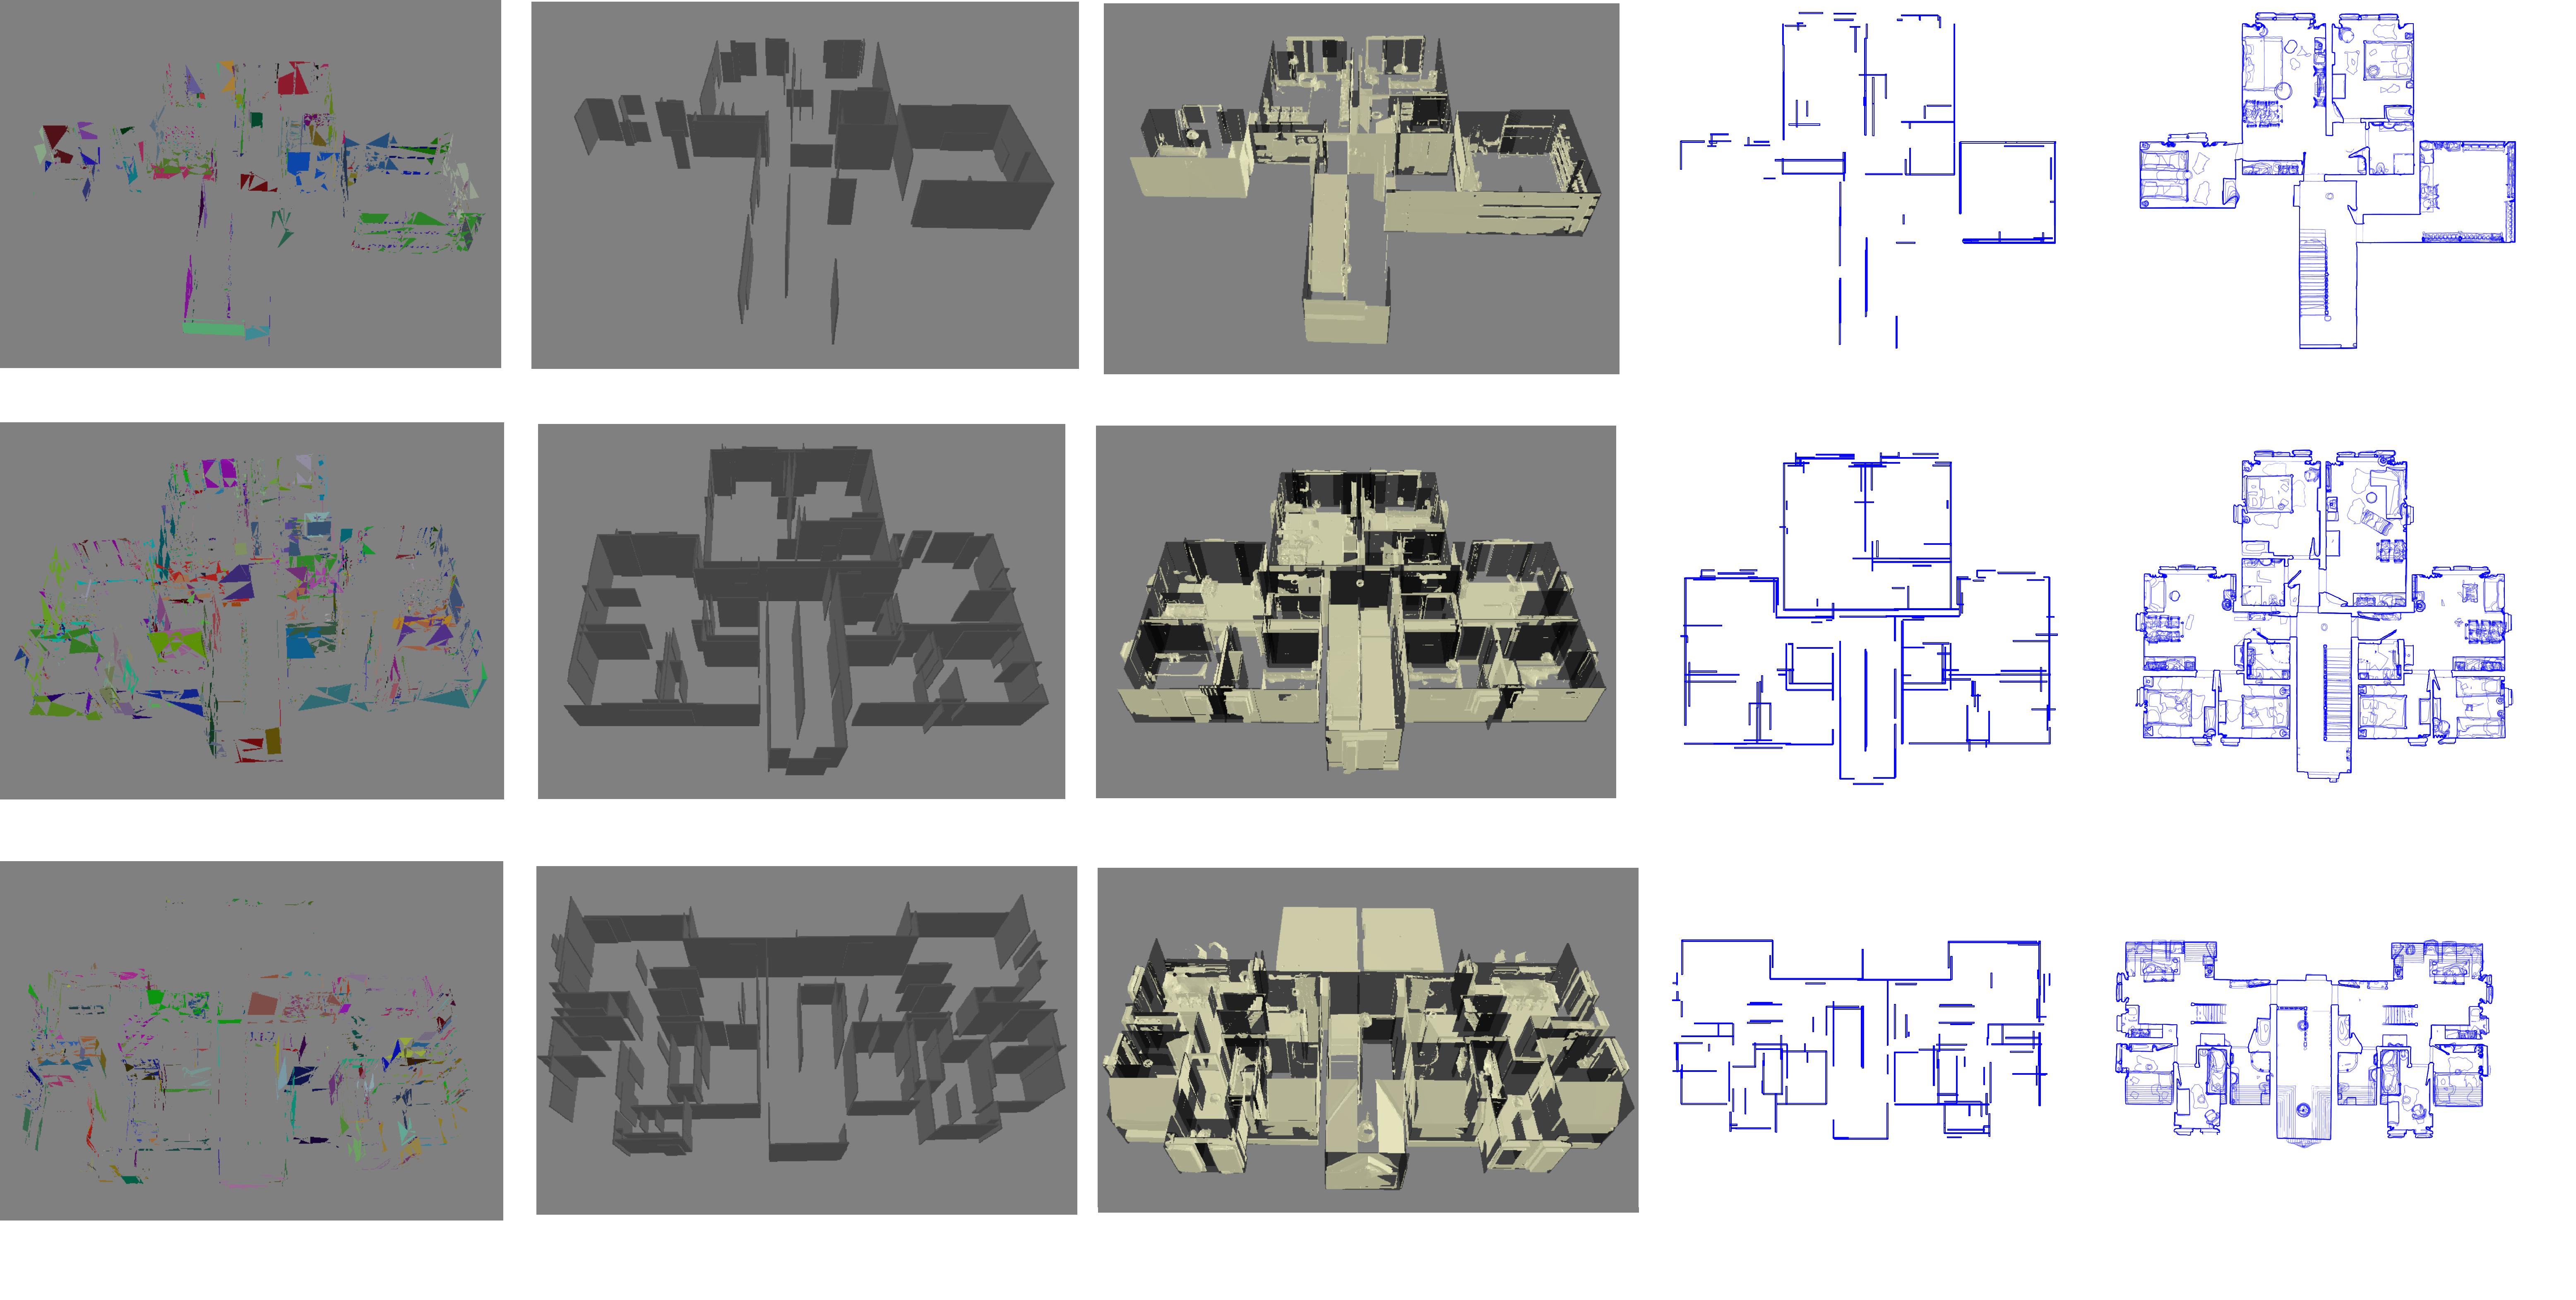}
  \centering
  \caption{Model 5: Left to right: Show clusters, flat walls, flat walls with building, drafting style  and pen-and-ink style floor plan for level 0 (top row) level 1 (middle row) and level 2 (bottom row). }
  \label{fig:matterport_level012_2}
\end{figure*}
